# Supplementary material for: On Deterministic Sketching and Streaming for Sparse Recovery and Norm Estimation
Source: arXiv:1206.5725 source file (2012-06-25)
Supplement: Supplementary file 1 [file appendix.tex]

\section{Inner Product with Tail Guarantee}
